# Supplementary material for: Neural Network-Driven Molecular Insights into Alkaline Wet Etching of GaN: Toward Atomistic Precision in Nanostructure Fabrication
Source: arXiv:2505.08165 ancillary file (2025-05-13)
Supplement: Supplementary file 1 [file Supporting_Information.pdf]

# Atomistic Mechanisms of GaN Wet Etching Unveiled by Neural-Network Potential Molecular Dynamics''

Purun-hanul Kim

Jeong Min Choi

Seungwu Han\*

Youngho Kang\*

Purun-hanul Kim, Jeong Min Choi,

Department of Materials Science and Engineering and Research Institute of Advanced Materials, Seoul National University, Seoul 08826, Republic of Korea

Prof. Seungwu Han

Department of Materials Science and Engineering and Research Institute of Advanced Materials, Seoul National University, Seoul 08826, Republic of Korea

Korea Institute for Advanced Study, Seoul 02455, Republic of Korea

Email Address: hansw@snu.ac.kr

Prof. Youngho Kang

Department of Materials Science and Engineering, Incheon National University, Incheon 22012, Republic of Korea

Email Address: youngho84@inu.ac.kr

## S1 BPNNP feature vectors and CUR decomposition

For the efficiency of training and inference of NNP, we select  $k$  features based on leverage score by single value decomposition of a full matrix ( $\mathbf{A}$ ) of 310 features by fully constructed Atom-centered symmetry functions (ACSFs) for the whole target training set. By constructing  $\mathbf{C}$  from the selected features for each element, the decomposition identifies the most important features for each element based on an error of  $\|\mathbf{A} - \mathbf{CUR}\|_2$  with threshold of 0.001, where  $\mathbf{U} = \mathbf{C}^* \mathbf{A} \mathbf{A}^*$ ,  $\mathbf{R} = \mathbf{A}$ , and  $(\cdot)^*$  denotes Moore-Penrose pseudo-inverse. The resulting parameters for symmetry functions for each element is summarized in Table S1. As a result, the final feature vector sizes become 145, 141, 51, 153, and 151 components for Ga, N, K, H, and O, respectively, as mentioned in main text.

Table S1: Parameters used in the symmetry functions for each central atom

| SF type | $e_c$ | $e_1$    | $e_2$ | $r_c$ (Å) | $\eta$ (Å <sup>-2</sup> )                        | $\lambda$ | $\zeta$ | # of SFs |
|---------|-------|----------|-------|-----------|--------------------------------------------------|-----------|---------|----------|
| $G_2$   | Ga    | Ga, N, O | -     | 6.0       | 0.003214, 0.071421, 0.214254, 0.714213, 1.428426 | -         | -       | 15       |
| $G_2$   | Ga    | H        | -     | 6.0       | 0.003214, 0.071421, 0.357106, 0.714213, 1.428426 | -         | -       | 5        |
| $G_2$   | Ga    | K        | -     | 6.0       | 0.003214, 0.124987, 0.357106, 1.428426           | -         | -       | 4        |
| $G_4$   | Ga    | Ga       | Ga    | 6.0       | 0.000357, 0.089277                               | 1, 2, 4   | 1, -1   | 8        |
| $G_4$   | Ga    | Ga       | H     | 6.0       | 0.000357, 0.028569, 0.089277                     | 1, 2, 4   | 1, -1   | 9        |
| $G_4$   | Ga    | Ga       | N     | 6.0       | 0.000357, 0.028569, 0.089277                     | 1, 2, 4   | 1, -1   | 9        |
| $G_4$   | Ga    | Ga       | O     | 6.0       | 0.000357, 0.028569, 0.089277                     | 1, 2, 4   | 1, -1   | 8        |

Table S1: (continued)

| SF type | $e_c$ | $e_1$    | $e_2$ | $r_c$ (Å) | $\eta$ (Å <sup>-2</sup> )                        | $\lambda$ | $\zeta$ | # of SFs |
|---------|-------|----------|-------|-----------|--------------------------------------------------|-----------|---------|----------|
| $G_4$   | Ga    | Ga       | K     | 6.0       | 0.000357, 0.028569, 0.089277                     | 1, 2, 4   | 1, -1   | 7        |
| $G_4$   | Ga    | H        | H     | 6.0       | 0.000357, 0.028569, 0.089277                     | 1, 2, 4   | 1, -1   | 8        |
| $G_4$   | Ga    | H        | N     | 6.0       | 0.000357, 0.028569, 0.089277                     | 1, 2, 4   | 1, -1   | 9        |
| $G_4$   | Ga    | H        | O     | 6.0       | 0.000357, 0.028569, 0.089277                     | 1, 2, 4   | 1, -1   | 8        |
| $G_4$   | Ga    | H        | K     | 6.0       | 0.000357, 0.028569, 0.089277                     | 1, 2, 4   | 1, -1   | 8        |
| $G_4$   | Ga    | N        | N     | 6.0       | 0.000357, 0.028569, 0.089277                     | 1, 2, 4   | 1, -1   | 9        |
| $G_4$   | Ga    | N        | O     | 6.0       | 0.000357, 0.028569, 0.089277                     | 1, 2, 4   | 1, -1   | 10       |
| $G_4$   | Ga    | N        | K     | 6.0       | 0.000357, 0.028569, 0.089277                     | 1, 2, 4   | 1, -1   | 8        |
| $G_4$   | Ga    | O        | O     | 6.0       | 0.000357, 0.028569, 0.089277                     | 1, 2, 4   | 1, -1   | 8        |
| $G_4$   | Ga    | O        | K     | 6.0       | 0.000357, 0.028569, 0.089277                     | 1, 2, 4   | 1, -1   | 7        |
| $G_4$   | Ga    | K        | K     | 6.0       | 0.000357, 0.028569, 0.089277                     | 1, 2, 4   | 1, -1   | 5        |
| $G_2$   | H     | Ga, H, O | -     | 6.0       | 0.003214, 0.124987, 0.357106, 0.714213, 1.428426 | -         | -       | 15       |
| $G_2$   | H     | N        | -     | 6.0       | 0.003214, 0.035711, 0.214264, 0.714213, 1.428426 | -         | -       | 5        |
| $G_2$   | H     | K        | -     | 6.0       | 0.003214, 0.071421, 0.214264, 0.714213, 1.428426 | -         | -       | 5        |
| $G_4$   | H     | Ga       | Ga    | 6.0       | 0.000357, 0.028569, 0.089277                     | 1, 2, 4   | 1, -1   | 7        |
| $G_4$   | H     | Ga       | H     | 6.0       | 0.000357, 0.028569, 0.089277                     | 1, 2, 4   | 1, -1   | 10       |
| $G_4$   | H     | Ga       | N     | 6.0       | 0.000357, 0.028569, 0.089277                     | 1, 2, 4   | 1, -1   | 7        |
| $G_4$   | H     | Ga       | O     | 6.0       | 0.000357, 0.028569, 0.089277                     | 1, 2, 4   | 1, -1   | 10       |
| $G_4$   | H     | Ga       | K     | 6.0       | 0.000357, 0.028569, 0.089277                     | 1, 2, 4   | 1, -1   | 7        |
| $G_4$   | H     | H        | K     | 6.0       | 0.000357, 0.028569, 0.089277                     | 1, 2, 4   | 1, -1   | 9        |
| $G_4$   | H     | H        | N     | 6.0       | 0.000357, 0.028569, 0.089277                     | 1, 2, 4   | 1, -1   | 8        |
| $G_4$   | H     | H        | O     | 6.0       | 0.000357, 0.028569, 0.089277                     | 1, 2, 4   | 1, -1   | 8        |

Table S1: (continued)

| SF type | $e_c$ | $e_1$   | $e_2$ | $r_c$ (Å) | $\eta$ (Å <sup>-2</sup> )                        | $\lambda$ | $\zeta$ | # of SFs |
|---------|-------|---------|-------|-----------|--------------------------------------------------|-----------|---------|----------|
| $G_4$   | H     | H       | K     | 6.0       | 0.000357, 0.028569, 0.089277                     | 1, 2, 4   | 1, -1   | 9        |
| $G_4$   | H     | N       | N     | 6.0       | 0.000357, 0.028569, 0.089277                     | 1, 2, 4   | 1, -1   | 9        |
| $G_4$   | H     | N       | O     | 6.0       | 0.000357, 0.028569, 0.089277                     | 1, 2, 4   | 1, -1   | 10       |
| $G_4$   | H     | N       | K     | 6.0       | 0.000357, 0.028569, 0.089277                     | 1, 2, 4   | 1, -1   | 8        |
| $G_4$   | H     | O       | O     | 6.0       | 0.000357, 0.028569, 0.089277                     | 1, 2, 4   | 1, -1   | 10       |
| $G_4$   | H     | O       | K     | 6.0       | 0.000357, 0.028569, 0.089277                     | 1, 2, 4   | 1, -1   | 9        |
| $G_4$   | H     | K       | K     | 6.0       | 0.000357, 0.028569, 0.089277                     | 1, 2, 4   | 1, -1   | 7        |
| $G_2$   | N     | Ga      | -     | 6.0       | 0.003214, 0.071421, 0.214254, 0.714213, 1.428426 | -         | -       | 5        |
| $G_2$   | N     | H, N, K | -     | 6.0       | 0.003214, 0.124987, 0.357106, 0.714213, 1.428426 | -         | -       | 15       |
| $G_2$   | N     | O       | -     | 6.0       | 0.003214, 0.071421, 0.357106, 0.714213, 1.428426 | -         | -       | 5        |
| $G_4$   | N     | Ga      | Ga    | 6.0       | 0.000357, 0.028569, 0.089277                     | 1, 2, 4   | 1, -1   | 7        |
| $G_4$   | N     | Ga      | H     | 6.0       | 0.000357, 0.028569, 0.089277                     | 1, 2, 4   | 1, -1   | 8        |
| $G_4$   | N     | Ga      | N     | 6.0       | 0.000357, 0.028569, 0.089277                     | 1, 2, 4   | 1, -1   | 7        |
| $G_4$   | N     | Ga      | O     | 6.0       | 0.000357, 0.028569, 0.089277                     | 1, 2, 4   | 1, -1   | 7        |
| $G_4$   | N     | Ga      | K     | 6.0       | 0.000357, 0.028569, 0.089277                     | 1, 2, 4   | 1, -1   | 8        |
| $G_4$   | N     | H       | H     | 6.0       | 0.000357, 0.028569, 0.089277                     | 1, 2, 4   | 1, -1   | 7        |
| $G_4$   | N     | H       | N     | 6.0       | 0.000357, 0.028569, 0.089277                     | 1, 2, 4   | 1, -1   | 7        |
| $G_4$   | N     | H       | O     | 6.0       | 0.000357, 0.028569, 0.089277                     | 1, 2, 4   | 1, -1   | 8        |
| $G_4$   | N     | H       | K     | 6.0       | 0.000357, 0.028569, 0.089277                     | 1, 2, 4   | 1, -1   | 8        |
| $G_4$   | N     | N       | N     | 6.0       | 0.000357, 0.028569, 0.089277                     | 1, 2, 4   | 1, -1   | 8        |
| $G_4$   | N     | N       | O     | 6.0       | 0.000357, 0.028569, 0.089277                     | 1, 2, 4   | 1, -1   | 9        |
| $G_4$   | N     | N       | K     | 6.0       | 0.000357, 0.028569, 0.089277                     | 1, 2, 4   | 1, -1   | 9        |

Table S1: (continued)

| SF type | $e_c$ | $e_1$ | $e_2$ | $r_c$ (Å) | $\eta$ (Å <sup>-2</sup> )                                  | $\lambda$ | $\zeta$ | # of SFs |
|---------|-------|-------|-------|-----------|------------------------------------------------------------|-----------|---------|----------|
| $G_4$   | N     | O     | O     | 6.0       | 0.000357, 0.028569, 0.089277                               | 1, 2, 4   | 1, -1   | 8        |
| $G_4$   | N     | O     | K     | 6.0       | 0.000357, 0.028569, 0.089277                               | 1, 2, 4   | 1, -1   | 8        |
| $G_4$   | N     | K     | K     | 6.0       | 0.000357, 0.028569, 0.089277                               | 1, 2, 4   | 1, -1   | 7        |
| $G_2$   | O     | Ga    | -     | 6.0       | 0.003214, 0.071421, 0.214254, 0.714213, 1.428426           | -         | -       | 5        |
| $G_2$   | O     | H     | -     | 6.0       | 0.003214, 0.071421, 0.214254, 0.357106, 0.714213, 1.428426 | -         | -       | 6        |
| $G_2$   | O     | N, K  | -     | 6.0       | 0.035711, 0.124987, 0.357106, 0.714213, 1.428426           | -         | -       | 10       |
| $G_2$   | O     | O     | -     | 6.0       | 0.003214, 0.124987, 0.357106, 0.714213, 1.428426           | -         | -       | 5        |
| $G_4$   | O     | Ga    | Ga    | 6.0       | 0.000357, 0.028569, 0.089277                               | 1, 2, 4   | 1, -1   | 8        |
| $G_4$   | O     | Ga    | H     | 6.0       | 0.000357, 0.028569, 0.089277                               | 1, 2, 4   | 1, -1   | 10       |
| $G_4$   | O     | Ga    | N     | 6.0       | 0.000357, 0.028569, 0.089277                               | 1, 2, 4   | 1, -1   | 8        |
| $G_4$   | O     | Ga    | O     | 6.0       | 0.000357, 0.028569, 0.089277                               | 1, 2, 4   | 1, -1   | 8        |
| $G_4$   | O     | Ga    | K     | 6.0       | 0.000357, 0.028569, 0.089277                               | 1, 2, 4   | 1, -1   | 8        |
| $G_4$   | O     | H     | H     | 6.0       | 0.000357, 0.028569, 0.089277                               | 1, 2, 4   | 1, -1   | 8        |
| $G_4$   | O     | H     | N     | 6.0       | 0.000357, 0.028569, 0.089277                               | 1, 2, 4   | 1, -1   | 8        |
| $G_4$   | O     | H     | O     | 6.0       | 0.000357, 0.028569, 0.089277                               | 1, 2, 4   | 1, -1   | 8        |
| $G_4$   | O     | H     | K     | 6.0       | 0.000357, 0.028569, 0.089277                               | 1, 2, 4   | 1, -1   | 9        |
| $G_4$   | O     | N     | N     | 6.0       | 0.000357, 0.028569, 0.089277                               | 1, 2, 4   | 1, -1   | 8        |
| $G_4$   | O     | N     | O     | 6.0       | 0.000357, 0.028569, 0.089277                               | 1, 2, 4   | 1, -1   | 9        |
| $G_4$   | O     | N     | K     | 6.0       | 0.000357, 0.028569, 0.089277                               | 1, 2, 4   | 1, -1   | 8        |
| $G_4$   | O     | O     | O     | 6.0       | 0.000357, 0.028569, 0.089277                               | 1, 2, 4   | 1, -1   | 8        |
| $G_4$   | O     | O     | K     | 6.0       | 0.000357, 0.028569, 0.089277                               | 1, 2, 4   | 1, -1   | 9        |
| $G_4$   | O     | K     | K     | 6.0       | 0.000357, 0.028569, 0.089277                               | 1, 2, 4   | 1, -1   | 8        |

Table S1: (continued)

| SF type | $e_c$ | $e_1$ | $e_2$ | $r_c$ (Å) | $\eta$ (Å <sup>-2</sup> )    | $\lambda$ | $\zeta$ | # of SFs |
|---------|-------|-------|-------|-----------|------------------------------|-----------|---------|----------|
| $G_2$   | K     | Ga, K | -     | 6.0       | 0.003214                     | -         | -       | 2        |
| $G_2$   | K     | H     | -     | 6.0       | 0.003214, 0.124987           | -         | -       | 2        |
| $G_2$   | K     | N, O  | -     | 6.0       | 0.003214, 0.071421           | -         | -       | 4        |
| $G_4$   | K     | Ga    | Ga    | 6.0       | 0.000357                     | 1         | -1      | 1        |
| $G_4$   | K     | Ga    | H     | 6.0       | 0.000357, 0.028569           | 1, 4      | 1, -1   | 4        |
| $G_4$   | K     | Ga    | N     | 6.0       | 0.000357, 0.028569           | 1         | 1, -1   | 3        |
| $G_4$   | K     | Ga    | O     | 6.0       | 0.000357, 0.028569           | 1         | 1, -1   | 3        |
| $G_4$   | K     | H     | H     | 6.0       | 0.000357, 0.028569           | 1, 4      | 1, -1   | 7        |
| $G_4$   | K     | H     | N     | 6.0       | 0.000357, 0.028569           | 1, 4      | 1, -1   | 4        |
| $G_4$   | K     | H     | O     | 6.0       | 0.000357, 0.028569, 0.089277 | 1, 2, 4   | 1, -1   | 8        |
| $G_4$   | K     | H     | K     | 6.0       | 0.000357, 0.028569           | 1,4       | 1,-1    | 4        |
| $G_4$   | K     | N     | N     | 6.0       | 0.000357                     | 1         | 1       | 1        |
| $G_4$   | K     | N     | O     | 6.0       | 0.000357                     | 1         | 1, -1   | 2        |
| $G_4$   | K     | N     | K     | 6.0       | 0.000357                     | 1         | 1       | 1        |
| $G_4$   | K     | O     | O     | 6.0       | 0.000357, 0.028569           | 1, 4      | 1, -1   | 4        |
| $G_4$   | K     | O     | K     | 6.0       | 0.000357, 0.028569, 0.089277 | 1, 2, 4   | 1, -1   | 1        |

## S2 Training set details

### S2.1 Reaction products

As mentioned in the main text, we generate molecular configurations of potential byproducts of alkaline wet etching using NVT-MD simulations. All supercells contain at least 100 atoms, which are initially distributed randomly within the cells with the cubic shape. For all cases, the cell density is chosen to represent both "high" and "low" density conditions. The target "high" or "low" densities are adjusted by  $\pm 1$  g/cm<sup>3</sup> by interpolating GaN (*s*), H<sub>2</sub>O (*aq*), and KOH (*s*) ambient densities based on the species ratio. In this way, we accommodate varying local structures during MD trajectories while maintaining consistent chemical reactant ratios. Subsequently, the temperature profiles follow melt-quench calculations to obtain amorphous GaN (4000K-3000K-300K), and sampling proceeds during the melting, quenching, and annealing steps. These trajectories represent the different chemically reacted structures observed during the etching simulation.

The stoichiometries are selected based on well-established chemical reaction equations for the alkaline wet etching of GaN as follows (Figure S1a and b):

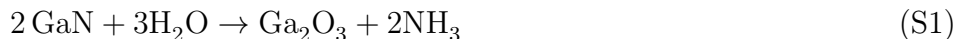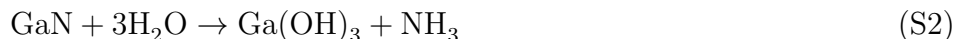

Additionally, we include excess  $m$  water molecules as dissolved species in the solution as shown in below equation (Figure S1c).

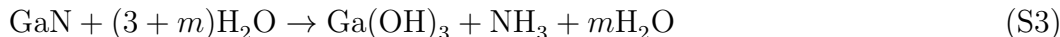

We further consider the GaN:H<sub>2</sub>O:KOH solution condition, as the presence of hydroxide ions imparts a negative charge to Ga hydroxide (Figure S1d and e).

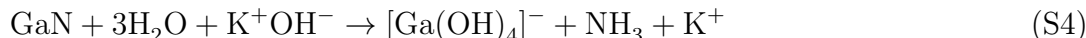

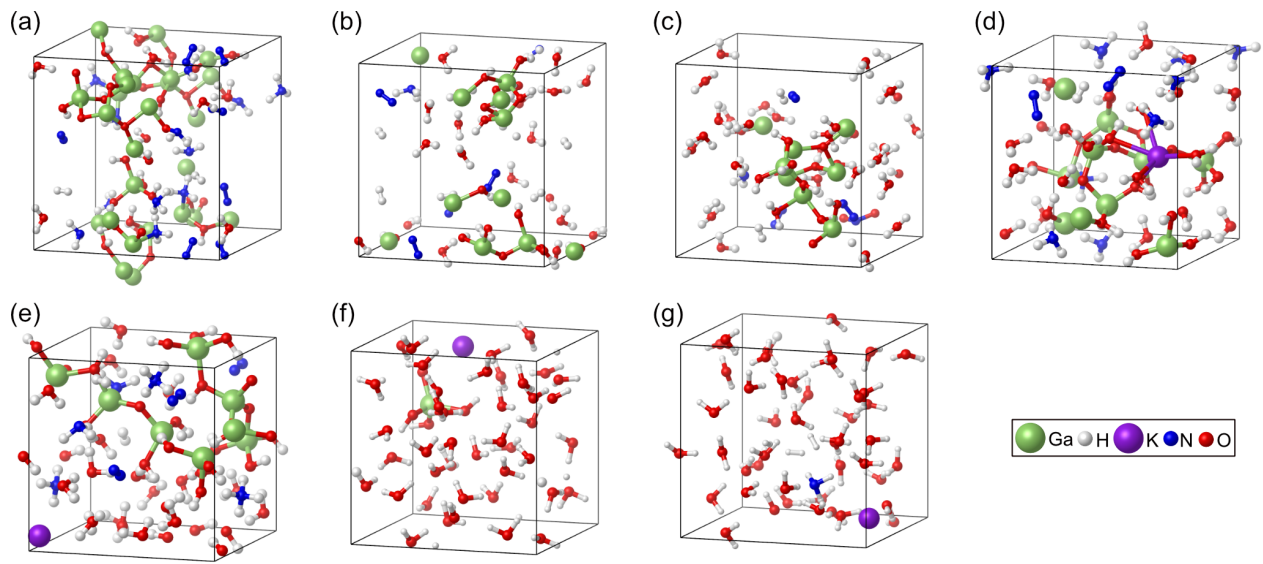

Figure S1: Atomic structures of final annealing step for each reaction. All structures represent the "low" density structure according to the linear interpolation of densities of GaN (*s*) and H<sub>2</sub>O (*aq*). (a) GaN:H<sub>2</sub>O=2:3 (b) GaN:H<sub>2</sub>O=1:3, (c) GaN:H<sub>2</sub>O=1:4, (d) GaN:KOH:H<sub>2</sub>O=1:1:3 (e) GaN:KOH:H<sub>2</sub>O=1:1:4, (f) [Ga(OH)<sub>4</sub>]<sup>−</sup> + K<sup>+</sup> + H<sub>2</sub>O and (g) NH<sub>3</sub> + K<sup>+</sup>OH<sup>−</sup> + H<sub>2</sub>O.

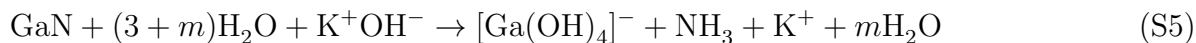

Furthermore, we conduct MD simulations with the same protocol for only one type of dissolved species in the bulk solution. We employ a single molecule of Ga hydroxide (eq S6) or ammonia (eq S7) in each bulk KOH solution, considering charge neutrality (Figure S1f and g).

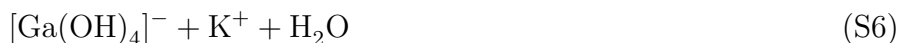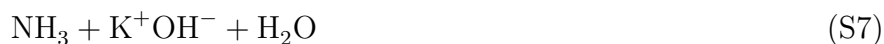

## S2.2 GaN/solution Interface

The GaN slab is constructed from a  $3 \times 2$  extension of the *m* plane, with a thickness of three bilayers. Initially, the structure is equilibrated using a NVT-MD simulation at 2000 K for the top-layer model and 600 K for the sublayer model for 3 ps, with no sampling during this step. The lower temperature is necessary for this initial equilibration step for the subsurface, as it is more reactive due to the presence of additional dangling bonds, which can lead to significant etching of the surface structure at higher temperatures. We confirm that no etching of GaN occurs during the equilibration steps. Subsequently, NPT-MD calculations are conducted for 5 ps at 100 kbar to determine solution volumes under the same pressure conditions as the etching simulations.

## S3 Iterative learning

### S3.1 Simulation details: Passivation and fixing

DFT calculations are performed on specific snapshots from the trajectories to select proper structures for iterative learning. To prevent charge transfer between the lower and upper planes in subsequent DFT calculations, the dangling bonds on the bottom surface must be appropriately passivated. The use of pseudo-hydrogen atoms with fractional charges, commonly used for passivation in DFT calculations, compromises the consistency between DFT and MLP results. As such, we employ H and OH species to passivate N and Ga dangling bonds, respectively. For the non-polar surfaces, as depicted in Figure S2a and

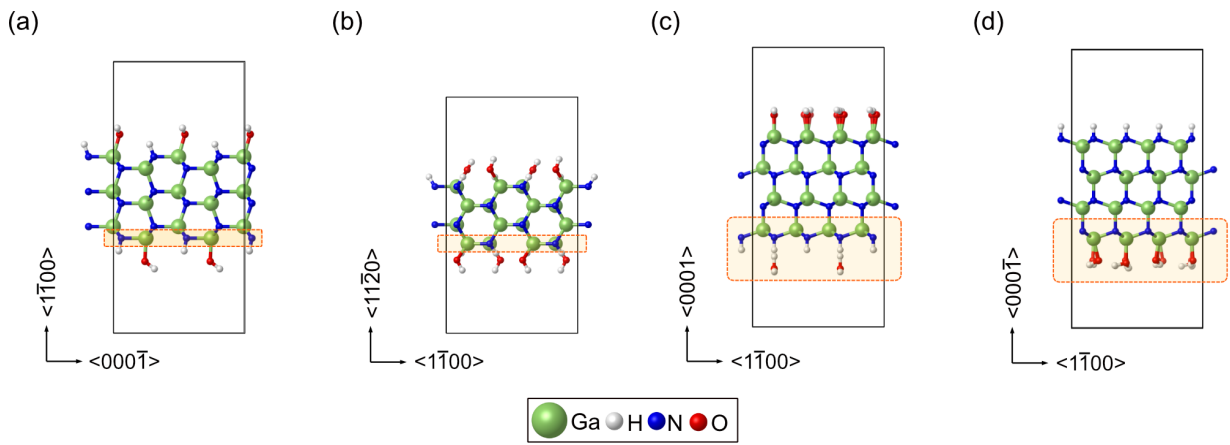

Figure S2: Atomic structures of target surfaces for MD simulations. Solution components (KOH) are omitted for clarity. The fixed regions are highlighted with orange boxes. (a)  $m$  plane, (b)  $a$  plane, (c)  $+c$  plane, and (d)  $-c$  plane

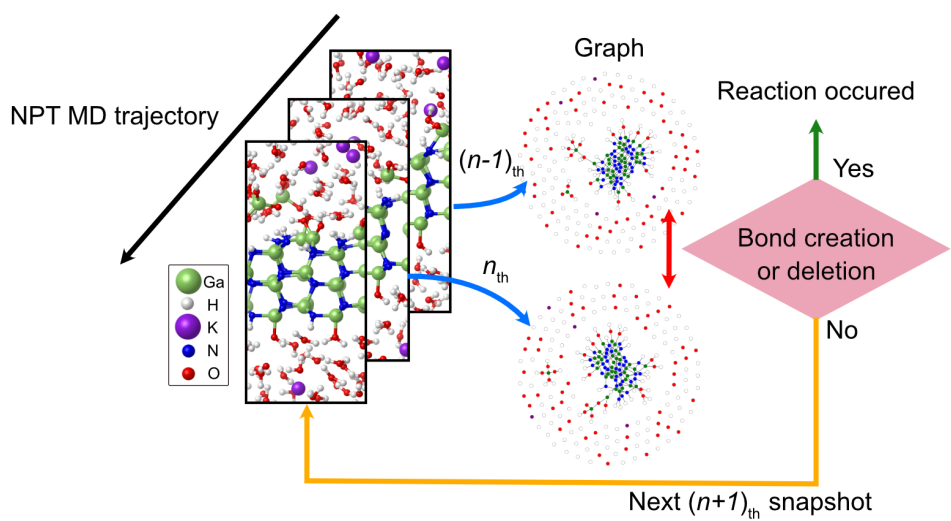

Figure S3: Schematic diagram of graph analysis of reaction moments during NNP-MD simulation.

b, all the dangling bonds on the top and bottom surfaces are fully passivated, and the atoms on the bottom surface are fixed. On the other hand, for the polar surfaces, only three-fourths of the dangling bonds are passivated to avoid introducing excess carriers into the system. Furthermore, the bottom surface is covered with fixed  $\text{H}_2\text{O}$  molecules to prevent chemical reactions due to the remaining unpassivated dangling bonds (Figure S2c and d).

### S3.2 Sampling snapshots using graph analysis

We identify reaction events through a graph analysis of the structures using **graph-tool**, which allows us to pinpoint the moments at which bond reorganization occurs, as illustrated in the Figure S3. Using graph analysis, the atoms and the bonds between the atoms are represented by graph nodes and edges, respectively. Therefore, comparing the graphs for each snapshot obtained from the MD trajectories, bond creation or deletion can be determined by whether edges are changed or not.

### S3.3 Evaluation of iterative learning

We evaluate atomic energies (eV/atom) for selected snapshots. When assessing atomic energies with the baseline NNP, we observe large energy error for untrained domain during etching of polar surfaces. Especially for the  $-c$  plane, there are large energy errors of over 100 meV/atom. Consequently, we conduct 3 iterative learning by improving atomic energy errors under 30 meV/atom (Figure S4b-d).

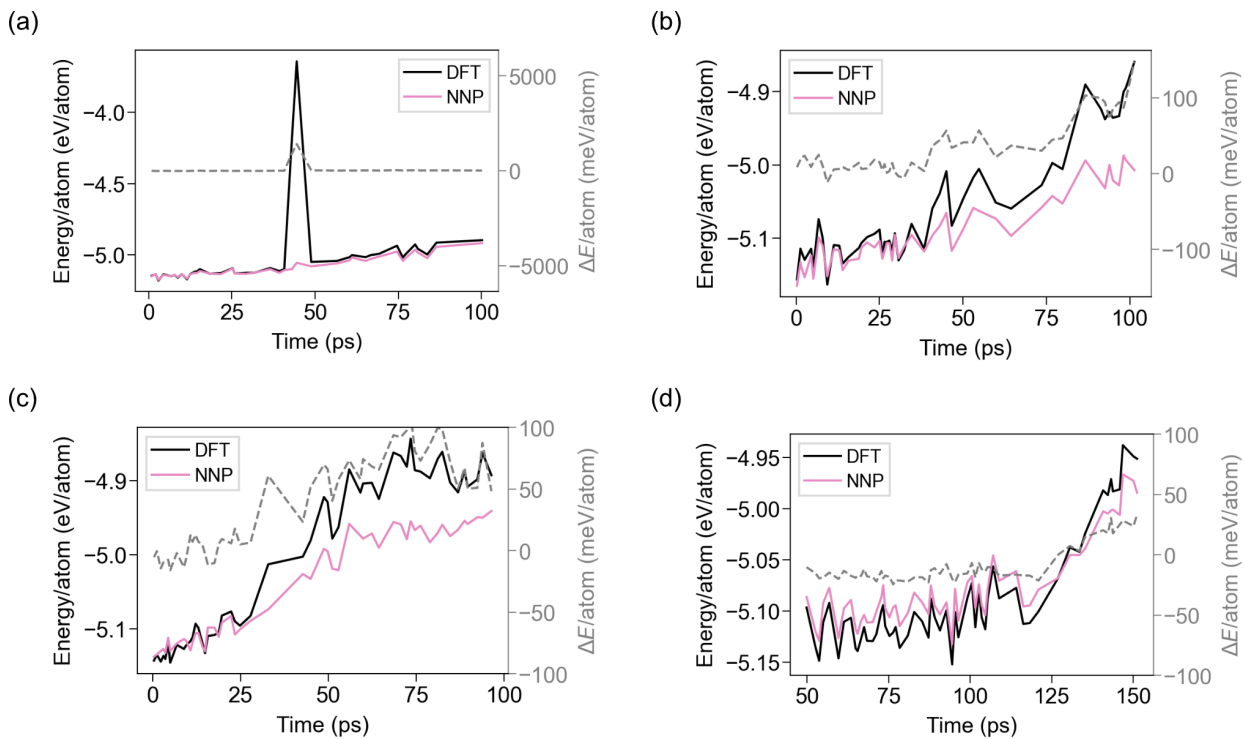

Figure S4: Procedure of iterative learning of  $-c$  plane. Each figure shows the total energies from DFT and NNP during the simulation time in eV/atom. The gray lines represent the differences between DFT and NNP, measured in meV/atom: (a) Baseline NNP, (b) after 1 iteration of learning, (c) after 2 iterations of learning, and (d) after 3 iterations of learning.

In addition to the evaluation of energy, we evaluated the distribution of force errors in box plots as shown in Figure S5. To investigate whether NNP well describes the reactions, we obtained the distribution of component force errors ( $|\Delta F|$ ) for all subsampled images. Subsequently, we evaluated mean absolute force errors (MAE), median and from third quartile to (Q3) to the maximum ( $Q3 + 1.5 \times IQR$ ) of force errors. The initial NNP shows large errors for some snapshots with force error larger than  $4 \text{ eV/\AA}$ , as shown in Figure S5a. However, after total 3 iterative learning, the MAE of force errors, as well as the deviation of errors indicated by Q3 and maximum, decreases and become uniform (Figure S5b-d).

## S4 Validation of NNP

### S4.1 Bulk properties

For bulk properties, we examine trivial properties such as the equation of state (EOS), relaxed structure properties, and elastic moduli (Figure S6a-d). Moreover, we compare NNP and DFT by radial distribution functions (RDFs) and vibrational density of states (VDOS) under high temperature, and high-pressure (2000 K and 100 kBar) conditions (Figure S6e-f).

### S4.2 Diffusivity of $\text{OH}^-$ in KOH solution

We examine the diffusivity of  $\text{OH}^-$  ion in KOH solution. For  $\text{OH}^-$ , the mean squared displacement (MSD) can be decomposed into two contributions, continuous and discrete MSD [1]. The continuous component arises from the vehicular motion of the hydroxide, while the discrete component results from the Grotthuss hopping mechanism.

Following the definition provided in the previous research [2] and with the hydroxide position defined as its center-of-mass, the total displacement over a time interval  $t$  (computed via a moving average over multiple time origins) is given by

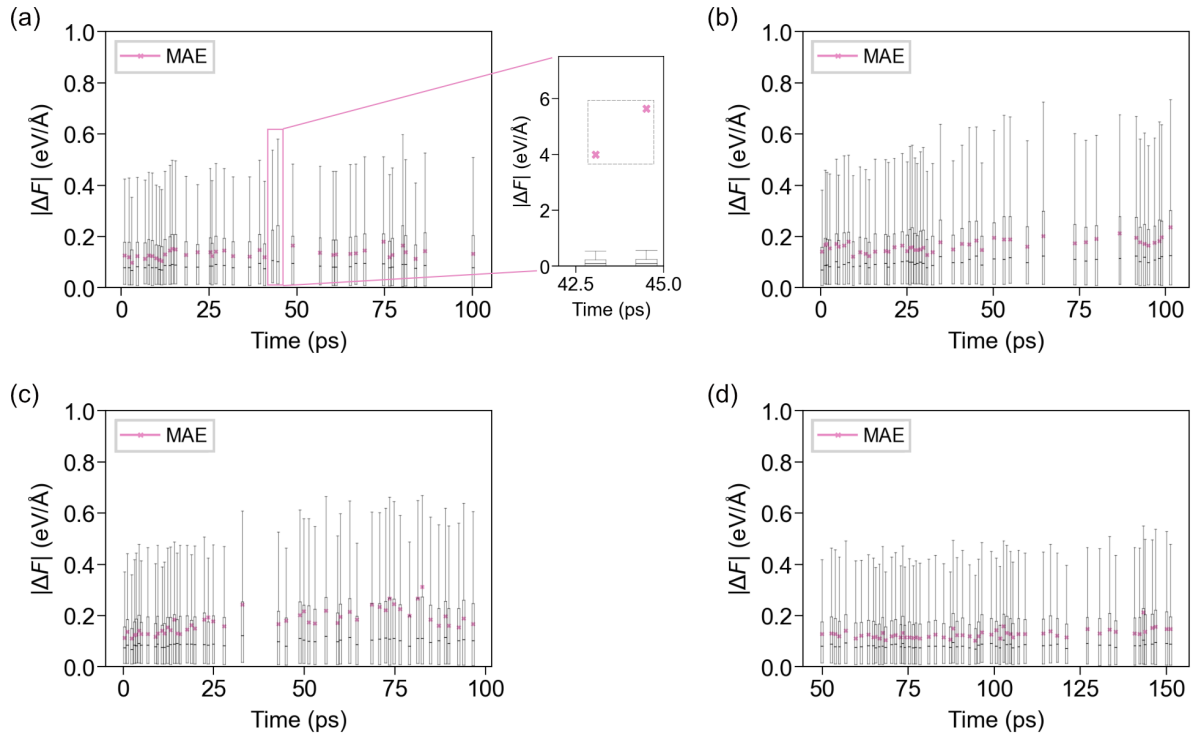

Figure S5: Procedure of evaluation of force errors during iterative learning of  $-c$  plane: (a) Baseline NNP, (b) after 1 iteration of learning, (c) after 2 iterations of learning, and (d) after 3 iterations of learning. Each figure shows the distribution for absolute component force errors ( $|\Delta F|$ ) between DFT and NNP in box plot format. The pink line represents mean absolute force error DFT and NNP, measured in  $\text{eV}/\text{\AA}$ .

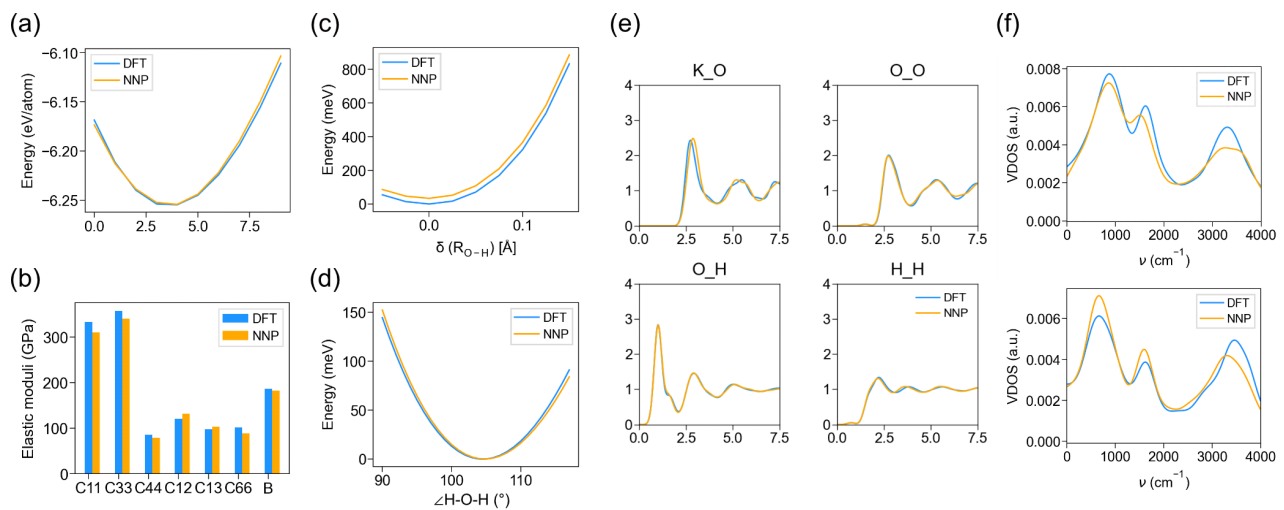

Figure S6: (a) Hydrostatic EOS of GaN, (b) Bulk moduli of GaN, (c) monomer EOS vs. OH bond length, (d) monomer water EOS vs. H-O-H angle, (e) RDF and (f) VDOS for bulk solution of KOH.

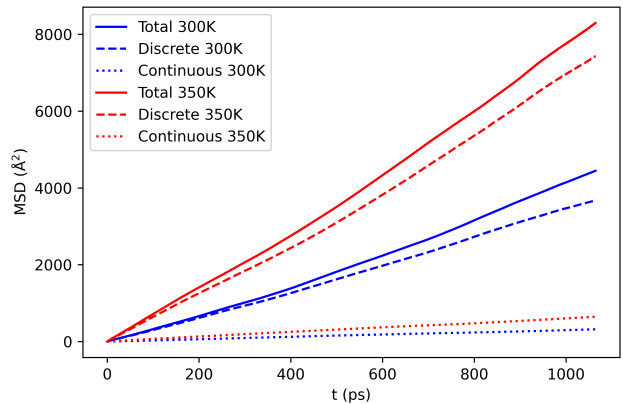

Figure S7: Enter Caption

$$\Delta \mathbf{r}(t) = \sum_{N'=1}^N \left[ P(t_{N'}) \Delta \mathbf{r}(t_{N'}) + (1 - P(t_{N'})) \Delta \mathbf{r}(t_{N'}) \right]$$

where, for a given time origin,  $t_{N'}$  denotes the time corresponding to the  $N'$ th frame. To distinguish between the contributions, the indicator function is introduced as

$$P(t_{N'}) = \begin{cases} 1, & \text{if the displacement at } t_{N'} \text{ corresponds to a discrete (hopping) event;} \\ 0, & \text{if the displacement at } t_{N'} \text{ is continuous (vehicular).} \end{cases}$$

The discrete and continuous contributions to the displacement are defined as

$$\Delta \mathbf{r}^{\text{dis}}(t) = \sum_{N'=1}^N P(t_{N'}) \Delta \mathbf{r}(t_{N'}),$$

$$\Delta \mathbf{r}^{\text{cont}}(t) = \sum_{N'=1}^N [1 - P(t_{N'})] \Delta \mathbf{r}(t_{N'}).$$

The corresponding MSD is expressed as

$$\text{MSD}_{\text{tot}}(t) = \langle \Delta \mathbf{r}(t)^2 \rangle = \langle \Delta \mathbf{r}^{\text{dis}}(t)^2 \rangle + \langle \Delta \mathbf{r}^{\text{cont}}(t)^2 \rangle + 2 \langle \Delta \mathbf{r}^{\text{dis}}(t) \cdot \Delta \mathbf{r}^{\text{cont}}(t) \rangle,$$

or equivalently,

$$\text{MSD}_{\text{tot}}(t) = \text{MSD}_{\text{dis}}(t) + \text{MSD}_{\text{cont}}(t) + 2 \text{MSD}_{\text{cross}}(t).$$

Diffusivity  $D$  is then determined from the Einstein relation:

$$\text{MSD}(t) = 6Dt.$$

For the molecular dynamics simulations, a simulation cell containing 925  $\text{H}_2\text{O}$  molecules and 8 KOH molecules (corresponding to a molality of approximately 0.48 kg/mol) was used. Two independent simulations were performed at each temperature (300 K and 350 K).

Table S2: Decomposed diffusivities ( $\text{\AA}^2/\text{ps}$ ) of hydroxide at 300 K and 350 K

| <b>T (K)</b> | <b>D<sub>total</sub></b> | <b>D<sub>dis</sub></b> | <b>D<sub>cont</sub></b> | <b>D<sub>Ref MD</sub> [3]</b> | <b>D<sub>Ref exp</sub> [4]</b> |
|--------------|--------------------------|------------------------|-------------------------|-------------------------------|--------------------------------|
| 300          | 0.768                    | 0.605                  | 0.050                   | 0.123                         | 0.527                          |
| 350          | 1.354                    | 1.220                  | 0.097                   | —                             | —                              |

Figure S7 and Table S2 clearly demonstrate that proton transfer is predominantly facilitated by the Grotthuss mechanism rather than by vehicular motion of hydroxide ions. This observation is consistent

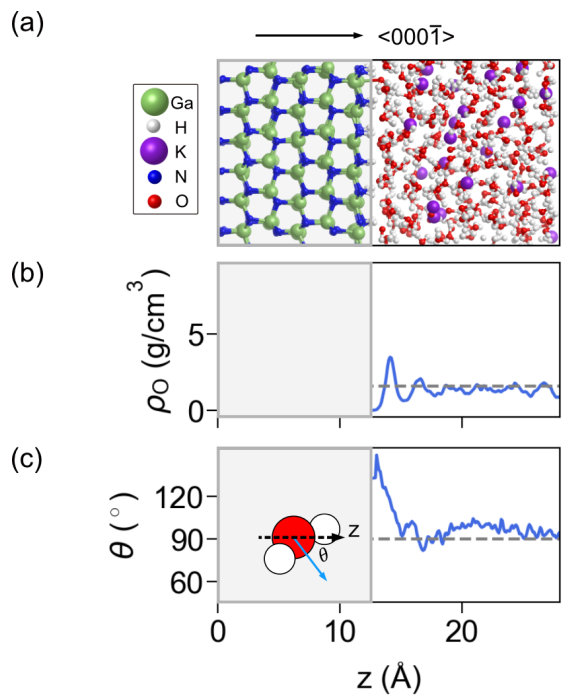

Figure S8: The example features of polar surface during the high pressure and temperature NNP-MD. (a) The atomic structure of GaN surface of  $-c$  plane and KOH aqueous solution. (b) The distribution of oxygen atom density in the solution cell. (c) The averaged angle distribution of water molecules in the solution with respect to  $z$ -axis. The angles are calculated between  $z$ -axis and polarity of the water molecule.

with the findings in the previous literature, [2] where hydroxide diffusivity was evaluated using ReaxFF in a tetramethylammonium hydroxide (TMAH) solution. In contrast, the low diffusivity reported in the different literature [3] can be attributed to the use of a non-reactive force field that does not capture the hopping mechanism during MD simulations.

### S4.3 Interface between GaN and KOH solution

To ensure the accuracy of our simulations involving the GaN surface-KOH solution interface, maintaining the neutrality of the bulk solution, away from the interfaces, is crucial. Polar surfaces, in particular, can significantly influence the solution, creating a thick electrical double layer (EDL). Additionally, due to the periodic boundary conditions (PBC) of the simulation cell, we carefully monitor interactions between interfaces to prevent them from compromising the neutrality of the bulk solution. While NNPs infer forces and energies based on local structural environments and may not fully account for long-range electrostatic interactions, we validate the solution's neutrality by examining the electrostatic potential exerted on the PBC cell through the water molecules' angle distribution, as illustrated in Figure S8 for the  $-c$  plane. In Figures S8a and b, oxygen atoms are located on the GaN top surface for Ga passivation and in the aqueous solution. At the interface, due to the orientation of the passivated hydroxide ions, nearby water molecules align with these ions, as depicted in Figure S8c. With a sufficient bulk solution thickness of 20 Å, the middle of the solution maintains an average angle of 90°, indicating a neutral bulk solution.

## S5 Etching simulation

### S5.1 Simulation details: Simulation cell

To investigate the evolution of morphologies during wet etching simulation, we used large cells to capture large-scale changes in the motifs. For each target surface, more than 800 formulas of GaN are used for GaN slabs as illustrated in the Tabel S3 . Furthermore, extra solution atoms are involved in the sim-

| Surface     | Slab size               | $a$ (Å) | $b$ (Å) | Number of GaN formula unit | Total atoms |
|-------------|-------------------------|---------|---------|----------------------------|-------------|
| + $c$ plane | $12 \times 12 \times 8$ | 44.30   | 41.56   | 864                        | 5076        |
| − $c$ plane | $12 \times 12 \times 8$ | 44.30   | 41.56   | 864                        | 4104        |
| $m$ plane   | $12 \times 8 \times 6$  | 38.37   | 41.56   | 1024                       | 5028        |
| $a$ plane   | $8 \times 8 \times 8$   | 44.30   | 41.56   | 1152                       | 4760        |

Table S3: Details of large-cell simulation for each surface

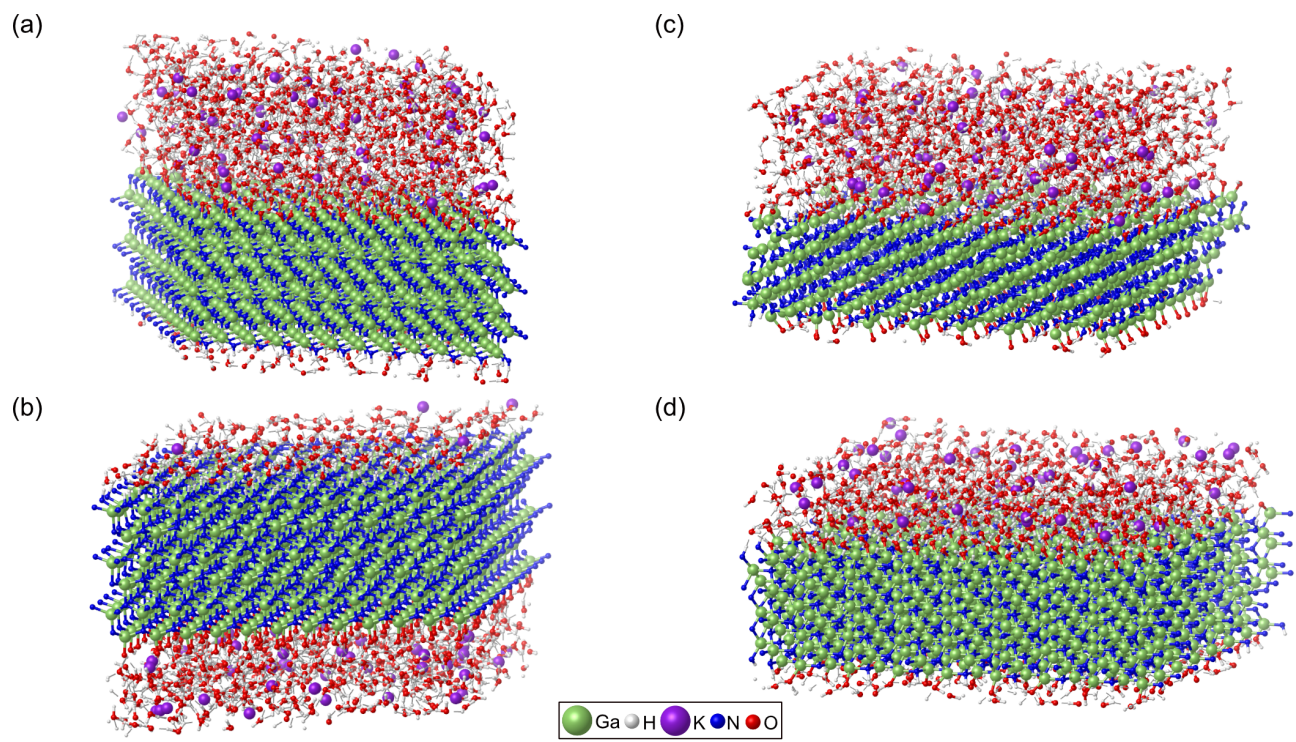Figure S9: Atomistic large cell structure of (a) + $c$  plane, (b) − $c$  plane, (c)  $m$  plane, and (d)  $a$  plane

ulation cell, making the solution slab thicker than the GaN one. The specific cell is illustrated in Figure S9.

## References

- [1] C. Chen, Y.-L. S. Tse, G. E. Lindberg, C. Knight, G. A. Voth, *Journal of the American Chemical Society* **2016**, *138*, 3 991, pMID: 26716727.
- [2] D. Dong, W. Zhang, A. C. T. van Duin, D. Bedrov, *The Journal of Physical Chemistry Letters* **2018**, *9*, 4 825, pMID: 29390610.
- [3] P. Habibi, A. Rahbari, S. Blazquez, C. Vega, P. Dey, T. J. H. Vlught, O. A. Moulτος, *The Journal of Physical Chemistry B* **2022**, *126*, 45 9376, pMID: 36325986.
- [4] L. Yuan-Hui, S. Gregory, *Geochimica et Cosmochimica Acta* **1974**, *38*, 5 703.

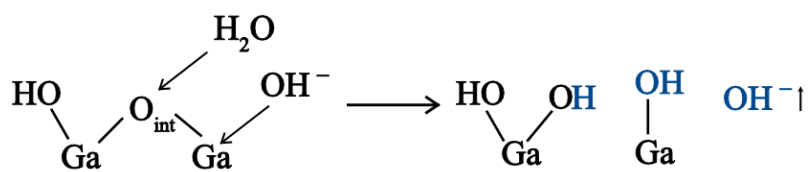

Figure S10: Chemical pathway to break  $\text{Ga-O}_{\text{int}}\text{-Ga}$  bonds with one water molecule and one  $\text{OH}^-$  ion. The reaction products are highlighted in blue.
